# Supplementary material for: 2D-3D Pose Tracking with Multi-View Constraints
Source: arXiv:2309.11335 source file (2023-09-20)
Supplement: Supplementary file 1 [file appendix.tex]

\begin{appendices}
\section{}
\label{sec:appendix}
% Here we present the detailed derivation for computing the Jacobians of quadrics factors. 
Following the notation convention of the paper, the quadric states in the world frame is represented by $(\mathbf{R}_q, \mathbf{t}_q, \mathbf{s}_q)$, and the robot pose is $(\mathbf{R}_r, \mathbf{t}_r)$. Therefore, the state vector involved in a single observation is $\mathbf{x} = [\mathbf{R}_r, \mathbf{t}_r, \mathbf{R}_q, \mathbf{t}_q, \mathbf{s}_q]$.

To simplify the presentation, we derive the Jacobian matrix based on a single observation, while the complete Jacobian can be constructed by filling in per observation Jacobians. 
% \section{Error Function}
As presented in the paper, the observation error is given by
\begin{equation}
    \begin{aligned}
    \mathbf{e} &= \begin{pmatrix}
        \mathbf{e}_{\mathbf{R}} \\ 
        \mathbf{e}_{\mathbf{t}} \\
        \mathbf{e}_{\mathbf{s}}
    \end{pmatrix}\\ &=\left(\begin{array}{l}
    \text{diag}(\mathbf{I^R}) \left(\mathbf{V} \otimes \mathbf{\Delta_R}\right)^T\\
    \text{diag}(\mathbf{I}^{\mathbf{t}}) (\mathbf{DV}^T\mathbf{\Delta_t+V}^T\mathbf{l})\\
    \text{diag}(\mathbf{I}^{\mathbf{s}}) (\mathbf{s}^2 - \mathbf{\Lambda})
    \end{array}\right)\in \mathbb{R}^{15}
    \end{aligned}
\end{equation}
where $\otimes$ means column-wise cross product. $\mathbf{\Delta}_\mathbf{R} = \mathbf{R}_r^T\mathbf{R}_q$ and $\mathbf{\Delta_t} = \mathbf{R}_r^T(\mathbf{t}_q - \mathbf{t}_r)$ are the rotation and translation of quadrics pose transformed into the robot frame. $\mathbf{\Lambda}=[\lambda_1,\lambda_2,\lambda_3]$ is the vector of eigenvalues which are stored as the diagonal elements of $\mathbf{D}$. Here, $\mathbf{e}_{\mathbf{R}}$ is a $3\times 3$ matrix and will be vectorized and then stacked into the error vector. 

Then we have the derivative $\frac{\partial \mathbf{e}}{\partial \mathbf{x}}\in \mathbb{R}^{15\times15}$ as 
\begin{equation}
    \dfrac{\partial \mathbf{e}}{\partial \mathbf{x}} = \begin{pmatrix} \dfrac{\partial \mathbf{e}_\mathbf{R}}{\partial \mathbf{R}_r} & \dfrac{\partial \mathbf{e}_\mathbf{R}}{\partial \mathbf{t}} & \dfrac{\partial \mathbf{e}_\mathbf{R}}{\partial \mathbf{R}_q} & \dfrac{\partial \mathbf{e}_\mathbf{R}}{\partial \mathbf{t}_q} & \dfrac{\partial \mathbf{e}_\mathbf{R}}{\partial \mathbf{s}_q}\\
    \dfrac{\partial \mathbf{e}_\mathbf{t}}{\partial \mathbf{R}_r} & \dfrac{\partial \mathbf{e}_\mathbf{t}}{\partial \mathbf{t}} & \dfrac{\partial \mathbf{e}_\mathbf{t}}{\partial \mathbf{R}_q} & \dfrac{\partial \mathbf{e}_\mathbf{t}}{\partial \mathbf{t}_q} & \dfrac{\partial \mathbf{e}_\mathbf{t}}{\partial \mathbf{s}_q} \\
    \dfrac{\partial \mathbf{e}_\mathbf{s}}{\partial \mathbf{R}_r} & \dfrac{\partial \mathbf{e}_\mathbf{s}}{\partial \mathbf{t}} & \dfrac{\partial \mathbf{e}_\mathbf{t}}{\partial \mathbf{R}_q} & \dfrac{\partial \mathbf{e}_\mathbf{s}}{\partial \mathbf{t}_q} & \dfrac{\partial \mathbf{e}_\mathbf{s}}{\partial \mathbf{s}_q}
    \end{pmatrix} 
\end{equation}
Note that the first dimension size 15 is the number of constraints or the error terms. The above Jacobian can be simplified by identifying zero blocks: 
\begin{equation}
    \dfrac{\partial \mathbf{e}}{\partial \mathbf{x}} = \begin{pmatrix} \dfrac{\partial \mathbf{e}_\mathbf{R}}{\partial \mathbf{R}_r} & \mathbf{0} & \dfrac{\partial \mathbf{e}_\mathbf{R}}{\partial \mathbf{R}_q} & \mathbf{0} & \mathbf{0}\\
    \dfrac{\partial \mathbf{e}_\mathbf{t}}{\partial \mathbf{R}_r} & \dfrac{\partial \mathbf{e}_\mathbf{t}}{\partial \mathbf{t}} & \dfrac{\partial \mathbf{e}_\mathbf{t}}{\partial \mathbf{R}_q} & \dfrac{\partial \mathbf{e}_\mathbf{t}}{\partial \mathbf{t}_q} & \mathbf{0} \\
    \mathbf{0} & \mathbf{0} & \mathbf{0} & \mathbf{0} & \dfrac{\partial \mathbf{e}_\mathbf{s}}{\partial \mathbf{s}_q}
    \end{pmatrix}
    \label{eqn:jacobian}
\end{equation}

Now we rewrite error terms explicitly to prepare for the derivation of $\frac{\partial \mathbf{e}}{\partial\mathbf{x}}$:
\begin{equation}
    \begin{aligned}
    \mathbf{e}_{\mathbf{R}} &= \begin{pmatrix} \cdots \\ [\mathbf{v}_i]_{\times}\mathbf{R}_r^T\mathbf{R}_q\mathbf{u}_i\\ \cdots \end{pmatrix} \in \mathbb{R}^{9\times 1} \\
    \mathbf{e}_{\mathbf{t}} &= \begin{pmatrix} \cdots \\ \lambda_i\mathbf{u}_i^T\mathbf{R}_q^T(\mathbf{t}_q-\mathbf{t}) +\mathbf{u}_i^T\mathbf{R}_q^T\mathbf{R}_r\mathbf{l} \\ \cdots \end{pmatrix} \in \mathbb{R}^{3\times 1}\\
    \mathbf{e}_{\mathbf{s}} &= \begin{pmatrix} \cdots \\ \mathbf{s}_i^2 - \lambda_i\\ \cdots \end{pmatrix} \in \mathbb{R}^{3\times 1} 
    \end{aligned}
\end{equation}
where $\mathbf{u}_i$ are unit vectors: 
\begin{equation}
    \mathbf{u}_1 = (1,0,0)^T, \;\mathbf{u}_2 = (0,1,0)^T, \;\mathbf{u}_3 = (0,0,1)^T
\end{equation}
\section{Linearization}
Computing Jacobian involving $\mathbf{R}_r$ and $\mathbf{R}_q$ requires linearization which can be achieved by applying the small angle approximation:
\begin{equation}
    \mathbf{R}_r = \mathbf{R}_r\delta \mathbf{R},\quad \delta\mathbf{R}_r\approx \mathbf{I} + [\mathbf{w}_r]_{\times}
\end{equation}
and
\begin{equation}
    \mathbf{R}_q = \mathbf{R}_q\delta \mathbf{R}_q,\quad \delta\mathbf{R}_q\approx \mathbf{I} + [\mathbf{w}_q]_{\times}
\end{equation}
where $[\cdot]_{\times}$ is the skew-symmetric operator:
\begin{equation}
    [\mathbf{w}]_{\times} = \begin{bmatrix} 0&-w_3&w_2\\w_3&0&-w1\\-w_2&w_1&0\end{bmatrix}
\end{equation}
and $\mathbf{I}$ is the identity matrix. Now we apply the anti-commutative rule of cross product
\begin{equation}
    \begin{aligned}
        &\mathbf{a}\times \mathbf{b} = [\mathbf{a}]_{\times}\mathbf{b} \\
        =&-\mathbf{b}\times\mathbf{a} = -[\mathbf{b}]_{\times} \mathbf{a}
    \end{aligned}\quad (\mathbf{a,b}\in\mathbb{R}^3)
\end{equation}
to linearize the error terms w.r.t. rotation $\mathbf{R}_r$ and $\mathbf{R}_q$:
\begin{equation}
    \begin{aligned}
    \Bar{\mathbf{e}}_\mathbf{R} \lvert_{\mathbf{R}_r}
    &= \begin{pmatrix} \cdots \\ [\mathbf{v}_i]_{\times}(\mathbf{I}+[\mathbf{w}_r]_{\times})^T\mathbf{R}_r^T\mathbf{R}_q\mathbf{u}_i\\ \cdots \end{pmatrix}\\
    &= \begin{pmatrix} \cdots \\ [\mathbf{v}_i]_{\times}(\mathbf{I}-[\mathbf{w}_r]_{\times})\mathbf{R}_r^T\mathbf{R}_q\mathbf{u}_i\\ \cdots \end{pmatrix}\\
    &= \begin{pmatrix} \cdots \\ [\mathbf{v}_i]_{\times}\mathbf{R}_r^T\mathbf{R}_q\mathbf{u}_i - [\mathbf{v}_i]_{\times}[\mathbf{w}_r]_{\times}\mathbf{R}_r^T\mathbf{R}_q\mathbf{u}_i\\ \cdots \end{pmatrix}\\
    &= \begin{pmatrix} \cdots \\ [\mathbf{v}_i]_{\times}\mathbf{R}_r^T\mathbf{R}_q\mathbf{u}_i + [\mathbf{v}_i]_{\times}[\mathbf{R}_r^T\mathbf{R}_q\mathbf{u}_i]_{\times}\mathbf{w}_r\\ \cdots \end{pmatrix}\\
    \end{aligned}
\end{equation}
\begin{equation}
    \begin{aligned}
    \Bar{\mathbf{e}}_\mathbf{R} \lvert_{\mathbf{R}_q}
    &= \begin{pmatrix} \cdots \\ [\mathbf{v}_i]_{\times}\mathbf{R}_r^T\mathbf{R}_q(\mathbf{I}+[\mathbf{w}_q]_{\times})\mathbf{u}_i\\ \cdots \end{pmatrix}\\
    &= \begin{pmatrix} \cdots \\ [\mathbf{v}_i]_{\times}\mathbf{R}_r^T\mathbf{R}_q\mathbf{u}_i+[\mathbf{v}_i]_{\times}\mathbf{R}_r^T\mathbf{R}_q[\mathbf{w}_q]_{\times}\mathbf{u}_i\\ \cdots \end{pmatrix}\\
    &= \begin{pmatrix} \cdots \\ [\mathbf{v}_i]_{\times}\mathbf{R}_r^T\mathbf{R}_q\mathbf{u}_i-[\mathbf{v}_i]_{\times}\mathbf{R}_r^T\mathbf{R}_q[\mathbf{u}_i]_{\times}\mathbf{w}_q\\ \cdots \end{pmatrix}\\
    \end{aligned}
\end{equation}

\begin{equation}
    \begin{aligned}
    \Bar{\mathbf{e}}_\mathbf{t} \lvert_{\mathbf{R}_r}
    &= \begin{pmatrix} \cdots \\ \lambda_i\mathbf{u}_i^T\mathbf{R}_q^T(\mathbf{t}_q-\mathbf{t})\\
        +\mathbf{u}_i^T\mathbf{R}_q^T\mathbf{R}_r(\mathbf{I}+[\mathbf{w}_r]_{\times})\mathbf{l} \\ \cdots \end{pmatrix} \\
    &= \begin{pmatrix} \cdots \\ \lambda_i\mathbf{u}_i^T\mathbf{R}_q^T(\mathbf{t}_q-\mathbf{t})\\
        +\mathbf{u}_i^T\mathbf{R}_q^T\mathbf{R}_r\mathbf{l} + \mathbf{u}_i^T\mathbf{R}_q^T\mathbf{R}_r[\mathbf{w}_r]_{\times}\mathbf{l} \\ \cdots \end{pmatrix} \\
    &= \begin{pmatrix} \cdots \\ \lambda_i\mathbf{u}_i^T\mathbf{R}_q^T(\mathbf{t}_q-\mathbf{t})\\
        +\mathbf{u}_i^T\mathbf{R}_q^T\mathbf{R}_r\mathbf{l} - \mathbf{u}_i^T\mathbf{R}_q^T\mathbf{R}_r[\mathbf{l}]_{\times}\mathbf{w}_r\\ \cdots \end{pmatrix} \\
    \end{aligned}
\end{equation}
\begin{equation}
    \begin{aligned}
    \Bar{\mathbf{e}}_\mathbf{t} \lvert_{\mathbf{R}_q}
    &= \begin{pmatrix} \cdots \\ \lambda_i\mathbf{u}_i^T(\mathbf{I}+[\mathbf{w}_r]_{\times})^T\mathbf{R}_q^T(\mathbf{t}_q-\mathbf{t})\\
        +\mathbf{u}_i^T(\mathbf{I}+[\mathbf{w}_r]_{\times})^T\mathbf{R}_q^T\mathbf{R}_r\mathbf{l} \\ \cdots \end{pmatrix} \\
    &= \begin{pmatrix} \cdots \\ \lambda_i\mathbf{u}_i^T(\mathbf{I}-[\mathbf{w}_r]_{\times})\mathbf{R}_q^T(\mathbf{t}_q-\mathbf{t})\\
        +\mathbf{u}_i^T(\mathbf{I}-[\mathbf{w}_r]_{\times})\mathbf{R}_q^T\mathbf{R}_r\mathbf{l} \\ \cdots \end{pmatrix} \\
    &= \begin{pmatrix} \cdots \\ -\lambda_i\mathbf{u}_i^T[\mathbf{w}_r]_{\times}\mathbf{R}_q^T(\mathbf{t}_q-\mathbf{t})\\
        -\mathbf{u}_i^T[\mathbf{w}_r]_{\times}\mathbf{R}_q^T\mathbf{R}_r\mathbf{l} +\cdots \\ \cdots \end{pmatrix} \\
    &= \begin{pmatrix} \cdots \\ \lambda_i\mathbf{u}_i^T[\mathbf{R}_q^T(\mathbf{t}_q-\mathbf{t})]_{\times}\mathbf{w}_r\\+\mathbf{u}_i^T[\mathbf{R}_q^T\mathbf{R}_r\mathbf{l}]_{\times}\mathbf{w}_r +\cdots \\ \cdots \end{pmatrix} \\
    \end{aligned}
\end{equation}

In the linearized cost function $\mathbf{e}_{\mathbf{t}}|_{\mathbf{R}_q}$, constant terms not related to $\mathbf{x}$ are omitted. The error terms are linearized in that now they are linear w.r.t. $\mathbf{w}_r$ and $\mathbf{w}_q$. Finally, from the above linearized equations, we can have the Jacobian blocks: 
\begin{equation}
    \begin{aligned}
    \frac{\partial \mathbf{e}_\mathbf{R}}{\partial \mathbf{R}_r} &= \begin{pmatrix} \cdots \\ [\mathbf{v}_i]_{\times}[\mathbf{R}_r^T\mathbf{R}_q\mathbf{u}_i]_{\times} \\ \cdots \end{pmatrix}\\
    \frac{\partial \mathbf{e}_\mathbf{t}}{\partial \mathbf{R}_r} &= \begin{pmatrix} \cdots \\- \mathbf{u}_i^T\mathbf{R}_q^T\mathbf{R}_r[\mathbf{l}]_{\times}\\ \cdots \end{pmatrix}\\
    \frac{\partial \mathbf{e}_{\mathbf{R}_r}}{\partial \mathbf{R}_q} &= \begin{pmatrix} \cdots \\-[\mathbf{v}_i]_{\times}\mathbf{R}_r^T\mathbf{R}_q[\mathbf{u}_i]_{\times}\\ \cdots \end{pmatrix}\\
    \frac{\partial \mathbf{e}_\mathbf{t}}{\partial \mathbf{R}_q} &= \begin{pmatrix} \cdots \\\lambda_i\mathbf{u}_i^T[\mathbf{R}_q^T(\mathbf{t}_q-\mathbf{t})]_{\times} +\mathbf{u}_i^T[\mathbf{R}_q^T\mathbf{R}_r\mathbf{l}]_{\times} \\ \cdots \end{pmatrix}\\
    \end{aligned}
\end{equation}

As to Jacobian w.r.t. translation and scale, it is straight forward: 
\begin{equation}
    \begin{aligned}
    \frac{\partial \mathbf{e}_\mathbf{t}}{\partial \mathbf{t}_r} &=  \begin{pmatrix} \cdots \\-\lambda_i\mathbf{u}_i^T\mathbf{R}_q^T\\ \cdots \end{pmatrix}\\
    \frac{\partial \mathbf{e}_\mathbf{t}}{\partial \mathbf{t}_q} &=  \begin{pmatrix} \cdots \\\lambda_i\mathbf{u}_i^T\mathbf{R}_q^T\\ \cdots \end{pmatrix}\\
    \frac{\partial \mathbf{e}_\mathbf{s}}{\partial \mathbf{s}_q} &= \begin{pmatrix} \cdots \\ 2\mathbf{s}_i\\ \cdots \end{pmatrix}
    \end{aligned}
\end{equation}
The computed Jacobian blocks can then be filled into (\ref{eqn:jacobian}) and finally used to construct the complete Jacobian matrix used in the LM method (see Algorithm \ref{alg:gn}). 

\end{appendices}
